# Supplementary material for: Efficient Distance Approximation for Structured High-Dimensional Distributions via Learning
Source: arXiv:2002.05378 source file (2020-02-14)
Supplement: Supplementary file 2 [file appendix_old.tex]

%!TEX root=main.tex

\appendix

\section{Learning algorithm for Bayesian Networks}\label{sec:app-bn}

In this section we give a learning algorithm for an unknown small indegree $\le d$ bayes nets $P$ over the sample space $\{0,1\}^n$ on a known graph $G$ on vertex set $[n]$. We take $m$ samples from this bayes net, $m$ to be fixed later. Our algorithm constructs a bayes net $Q$ on $G$ as follows. It looks at the samples where the parents of $i$ is $a$, and the empirical distribution $Q(i\mid a)$ defined at node $i$ by these samples is used as the conditional distribution of $i$ when its parents are $a$. If no sample has parents of $i$ as $a$, then we define this conditional distribution arbitrarily, say the uniform bit. Let $P(i \mid a)$ be the true conditional distribution.
   
For every vertex $i$, for every fixing $a$ of its parents, let $\Pi[i,a]$ denote the event that parents of $i$ takes value $a$. We call a tuple $(i,a)$ {\em heavy} if $P[\Pi[i,a]]\ge \epsilon^2/n\cdot 2^d$ and {\em light} otherwise. Then if $m \ge 8n \cdot 2^d \ln (n 2^d)/\epsilon^2$ for every heavy tuple $(i,a)$ number of samples where parents of $i$ is $a$ is at least $m\cdot P[\Pi_{i,a}]/2 \ge 1$ except for 1/20 probability from Chernoff's and union bounds. We henceforth condition on this event $E$.

We use the following inequality from~\cite{10.5555/3327546.3327691} for bounding the Hellinger distane between two bayes nets on the same graph.
\begin{theorem}
$H^2(P,Q) \le \sum_i \sum_a \sqrt{P[\Pi_{i,a}]Q[\Pi_{i,a}]} H^2(P(i\mid a),Q(i\mid a))$
\end{theorem}

We get $H^2(P,Q) \le {1\over 2}\sum_i \sum_a P[\Pi_{i,a}] H^2(P(i\mid a),Q(i\mid a))+{1\over 2}\sum_i \sum_a Q[\Pi_{i,a}] H^2(P(i\mid a),Q(i\mid a))$ from AM-GM inequality and upper bound the expected value of the two terms separately under random sampling (conditioned on $E$).

For the first term:
\begin{align*}
&\ex{\sum_i \sum_a P[\Pi_{i,a}] H^2(P(i\mid a),Q(i\mid a))}\\
&=\sum_{(i,a)\text{ light}} P[\Pi_{i,a}] \ex{H^2(P(i\mid a),Q(i\mid a))}+\sum_{(i,a)\text{ heavy}} P[\Pi_{i,a}] \ex{H^2(P(i\mid a),Q(i\mid a))}\\
&\le \sum_{(i,a)\text{ light}} \epsilon^2/n\cdot 2^d + \sum_{(i,a)\text{ heavy}} P[\Pi_{i,a}] \ex{{(P(i=0\mid a)-Q(i=0\mid a))^2\over P(i=0\mid a)}+{(P(i=1\mid a)-Q(i=1\mid a))^2\over P(i=1\mid a)}}\\
\end{align*}

For the heavy tuples since we have seen at least $m\cdot P[\Pi_{i,a}]/2 \ge 1$ samples, from variance argument  $\ex{(P(i=0\mid a)-Q(i=0\mid a))^2/P(i=0\mid a)} \le 2P(i=0\mid a)(1-P(i=0\mid a))/m \cdot P[\Pi_{i,a}] \cdot P(i=0\mid a)$, similarly for the $i=1$ case. Plugging in the last equation we get, 
\begin{align*}
&\ex{\sum_i \sum_a P[\Pi_{i,a}] H^2(P(i\mid a),Q(i\mid a))}\\
&\le \sum_{(i,a)} \max\{\epsilon^2/n\cdot 2^d,2/m\}\\
&\le \epsilon^2
\end{align*}

The analysis of the second term is more complicated since $Q[\Pi_{i,a}]$ is a random variable.

\begin{align*}
&\ex{\sum_i \sum_a  Q[\Pi_{i,a}] H^2(P(i\mid a),Q(i\mid a))}\\
&=\sum_{(i,a)\text{ light}} \ex{Q[\Pi_{i,a}] H^2(P(i\mid a),Q(i\mid a))}+\sum_{(i,a)\text{ heavy}} \ex{Q[\Pi_{i,a}] H^2(P(i\mid a),Q(i\mid a))}\\
&\le \sum_{(i,a)\text{ light}} \ex{Q[\Pi_{i,a}]}+\sum_{(i,a)\text{ heavy}} \ex{Q[\Pi_{i,a}] H^2(P(i\mid a),Q(i\mid a))}\\
\end{align*}

The random variables $Q[\Pi_{i,a}]$ and $H^2(P(i\mid a),Q(i\mid a))$ are not independent. Nevertheless for the heavy items due to bayes net topological order and our algorithm design, upon conditioning of the event $Q[\Pi_{i,a}]=t$ for any $t$, the conditional distribution of $Q(i\mid a)$ remains the same as the unconditional distribution. This is because for the heavy items at least one sample with parents of $i$ as $a$ is seen. Thus we can upper bound the previous expression similarly as before.

\begin{align*}
&\ex{\sum_i \sum_a  Q[\Pi_{i,a}] H^2(P(i\mid a),Q(i\mid a))}\\
&\le \sum_{(i,a)\text{ light}} \ex{Q[\Pi_{i,a}]}+\sum_{(i,a)\text{ heavy}} {2\over m \cdot P[\Pi_{i,a}]}\ex{Q[\Pi_{i,a}]}\\
\end{align*}

The expectation of the marginal distribution $\ex{Q[\Pi_{i,a}]}$ is harder to analyze since we might be using arbitrary distribution at a node topological order before the parents of $i$ due to lack of samples. 

\begin{align*}
&\sum_{(i,a)\text{ heavy}} \ex{Q[\Pi_{i,a}]}/P[\Pi_{i,a}]\\
&=\sum_{(i,a)\text{ heavy}} \sum_t \ex{Q[\Pi_{i,a}\circ t]}/P[\Pi_{i,a}]\\
\end{align*}

where $t$ varies over all possible assignments for nodes other than parents of $a$. The joint assignments $\Pi_{i,a}\circ t$ are of two kinds: 1) every parent setting is heavy in the assignment (recall $(i,a)$ itself is heavy) 2) there exists at least 1 light parent setting in the assignment. Let $H$ and $L$ be these two sets of assignments for $t$ respectively. We upper bound the previous expression.

\begin{align*}
&\sum_{(i,a)\text{ heavy}} \ex{Q[\Pi_{i,a}]}/P[\Pi_{i,a}]\\
&=\sum_{(i,a)\text{ heavy}} (\sum_{t\in H} \ex{Q[\Pi_{i,a}\circ t]}/P[\Pi_{i,a}]+\sum_{t\in L} \ex{Q[\Pi_{i,a}\circ t]}/P[\Pi_{i,a}])\\
\end{align*}

If $\sum_{t\in H}$ then in every parent setting of $Q[\Pi_{i,a}]\circ t$ at least 1 sample is seen. Hence due to bayes net topological order and our algorithm design, $\ex{Q[\Pi_{i,a}]\circ t}=P[\Pi_{i,a}]\circ t$. For $\sum_{t\in L}$ we have:
\begin{align*}
&\sum_{(i,a)\text{ heavy}} \sum_{t\in L} \ex{Q[\Pi_{i,a}\circ t]}/P[\Pi_{i,a}]\\
\end{align*}

Let $H'\subseteq \{0,1\}^n$ be the set of assignments of the complete distribution where every parent setting is heavy and let $L'$ be the rest. We claim that $\sum_{x\in L'} \ex{Q[x]} \le \epsilon^2$. This is because, for every $x\in L'$ we collect terms at the earliest light setting in the topological order, say parents of $i'=a$ and marginalize out all variables afterwards in $Q$. Since every setting before $i'=a$ is heavy, in expectation we can replace the $Q$ by $P$. Finally we marginalize out all variables except $i'$s parents in $P$. We shall be left with $P[\text{earliest light setting}] \le \epsilon^2/n\cdot 2^d$. Since we have at most $n\cdot 2^d$ collection points, the $\epsilon^2$ upper bound follows.

For any fixed $i$, $\sum_{a: \text{ (i,a) heavy}} \sum_{t \in L } \ex{Q[\Pi_{i,a}\circ t]} \le \sum_{x\in L'} \ex{Q[x]} \le \epsilon^2$. Summing over the $n$ values of $i$ we have:
\begin{align*}
&\sum_{(i,a)\text{ heavy}} \sum_{t\in L} \ex{Q[\Pi_{i,a}\circ t]}/P[\Pi_{i,a}]\\
&\le {n^2\cdot 2^d}
\end{align*}
using heaviness of $P[\Pi_{i,a}]$ and the $\epsilon^2$ upper bound.

We get:
\begin{align*}
&\sum_{(i,a)\text{ heavy}} \ex{Q[\Pi_{i,a}]}/P[\Pi_{i,a}]\\
&=\sum_{(i,a)\text{ heavy}} (\sum_{t\in H} \ex{Q[\Pi_{i,a}\circ t]}/P[\Pi_{i,a}]+\sum_{t\in L} \ex{Q[\Pi_{i,a}\circ t]}/P[\Pi_{i,a}])\\
&\le \sum_{(i,a)\text{ heavy}} \sum_{t\in H} P[\Pi_{i,a}\circ t]/P[\Pi_{i,a}] +{n^2\cdot 2^d}\\
&\le \sum_{(i,a)\text{ heavy}} 1 +{n^2\cdot 2^d}\\
&\le n\cdot 2^d + n^2 \cdot 2^d
\end{align*}

The term $\sum_{(i,a)\text{ light}} \ex{Q[\Pi_{i,a}]}$ can be upper bounded by $n\epsilon^2$ similarly since in this case every setting $Q[\Pi_{i,a}]\circ t$ is light. Finally we have:
\begin{align*}
&\ex{\sum_i \sum_a  Q[\Pi_{i,a}] H^2(P(i\mid a),Q(i\mid a))}\\
&\le \sum_{(i,a)\text{ light}} \ex{Q[\Pi_{i,a}]}+\sum_{(i,a)\text{ heavy}} {2\over m \cdot P[\Pi_{i,a}]}\ex{Q[\Pi_{i,a}]}\\
&\le n\epsilon^2 + {2\over m} (n\cdot 2^d + n^2 \cdot 2^d)\\
&\le 2n\epsilon^2 
\end{align*}
for $m \ge  8n \cdot 2^d/\epsilon^2$. 

Together we get $\ex{H^2(P,Q)}\le 2n\epsilon^2$ conditioned on the event $E$. From Markov's inequality and $Pr[E]\ge 19/20$ we get with at least 2/3 probability $H(P,Q) \le 2\sqrt{2n}\epsilon$ for $m \ge 8n \cdot 2^d \ln (n 2^d)/\epsilon^2$. Therefore $O(n^22^d\ln (n2^d)/\epsilon^2)$ samples achieve $H(P,Q)\le \epsilon$.
